# Supplementary material for: Simplicial SMOTE: Oversampling Solution to the Imbalanced Learning Problem
Source: arXiv:2503.03418 source file (2025-03-05)
Supplement: Supplementary file 1 [file appendix.tex]

\appendix

\section{Datasets summary}
\input{tables/datasets}

\clearpage
\onecolumn
\section{Sensitivity to hyperparameters}
\label{appendix_sensitivity}
\vspace{-0.5em}
\input{figures/sensitivity_simplicial_knn}

\clearpage
\section{Matthew's Correlation Coefficients}
\label{appendix_more_results}

\input{tables/results_knn_mcc}
\input{tables/results_gb_mcc}
